# Supplementary material for: Multilayer Structures of Graphene and Pt Nanoparticles -- a Multiscale Computational Study
Source: arXiv:2004.12107 source file (2020-04-25)
Supplement: Supplementary file 1 [file supporting_information.pdf]

## Appendix A: Solution of the elastic model for a deformed graphene sheet

We consider the following elastic boundary value problem: A thin membrane of planar modulus of elasticity $E_{2D}$ and Poisson number $\nu$ is, along a circle of radius $R_\mathrm{p}$ around the origin, perpendicularly displaced by a distance $h$, hence, $u_z(r = R_\mathrm{p}) = 0$. The membrane is clamped along a second circle of radius $R_\mathrm{d}$ where $u_z(r = R_\mathrm{d}) = h$. In addition, we assume that $u_r(r = R_\mathrm{p}) = u_r(r = R_\mathrm{d}) = 0$.

The stresses in radial and tangential directions are related to the radial and tangential strains by

$$\sigma_{rr} = E_{2D}\left(\epsilon_{rr} + \nu\epsilon_{\theta\theta}\right) \qquad \sigma_{\theta\theta} = E_{2D}\left(\epsilon_{\theta\theta} + \nu\epsilon_{rr}\right) \tag{1}$$

where $E_{2D}$ is the two-dimensional Young's modulus, $\nu$ Poisson's ratio for graphene and $\epsilon_{rr}$ and $\epsilon_{\theta\theta}$ are the radial and tangential strains. The stress equilibrium conditions for this cylindrically symmetric problem are, in cylindrical coordinates, given by

$$\frac{\partial\sigma_{rr}}{\partial r} + \frac{\sigma_{rr} - \sigma_{\theta\theta}}{r} = 0, \qquad \frac{\partial\sigma_{\theta\theta}}{\partial\theta} = 0 \tag{2}$$

To solve this problem, we follow Ref. [1] and start out from the assumption that the radial displacements (which are constrained to be zero on the outer and inner circle) are negligible in comparison with the displacements in $z$ direction.

$$u_r << u_z \quad , \quad \partial_r u_r \ll \partial_r u_z \tag{3}$$

Under this assumption, $\epsilon_{\theta\theta}$ is negligible, which leads to:

$$\frac{\partial\epsilon_{rr}}{\partial r} + \frac{1}{r}\epsilon_{rr}\left(1 - \nu\right) = 0 \tag{4}$$

Also, since $u_r$ is small, the radial extension $\mathrm{d}\rho$ of a membrane segment of extension $\mathrm{d}r$ in the undeformed configuration is, in the deformed configuration, approximately given by $\mathrm{d}\rho = \mathrm{d}r\sqrt{1 + (\mathrm{d}u_z/\mathrm{d}r)^2} \approx 1 + (1/2)(\mathrm{d}u_z/\mathrm{d}r)^2$ from which the radial stretch of the sheet follows as

$$\epsilon_{rr} = \frac{1}{2}\left(\frac{\partial u_z}{\partial r}\right)^2 \tag{5}$$

which leads us to the differential equation

$$\frac{\partial^2 u_z}{\partial r^2} + \frac{1 - \nu}{2r}\frac{\partial u_z}{\partial r} = 0 \tag{6}$$

The radial change of $u_z$ is determined by the factor $a = 1 - \frac{1-\nu}{2}$. A considerable algebraic simplification is obtained by setting $\nu \approx 1/3$ which leads to the numerical approximation

$$a = \frac{1 + \nu}{2} \approx \frac{2}{3} \tag{7}$$

Accounting for the boundary conditions at $r = R_\mathrm{p}$ and $r = R_\mathrm{d}$ we obtain the following solutions:

$$u_z = h\frac{R_\mathrm{d}^{2/3} - r^{2/3}}{R_\mathrm{d}^{2/3} - R_\mathrm{p}^{2/3}} \qquad \epsilon_{rr} = \frac{2h^2}{9}\frac{r^{-2/3}}{(R_\mathrm{d}^{2/3} - R_\mathrm{p}^{2/3})^2} \tag{8}$$

The elastic energy can then be written as:

$$E_{\rm el} = \frac{2\pi}{27} E_{2D} \frac{h^4}{(R_{\rm d}^{2/3} - R_{\rm p}^{2/3})^3} = \pi R_p^2 \frac{2E_{2D}}{27} \frac{q_p^4}{(q_{\rm p}^{2/3} - 1)^3} \tag{9}$$

where in the last step we have introduced the non-dimensional ratios $q_{\rm p} = h/R_{\rm p}$ and $q_{\rm d} = R_{\rm d}/R_{\rm p}$.

[1] Begley, M. R. & Mackin, T. J. Spherical indentation of freestanding circular thin films in the membrane regime. *J. Mech. Phys. Solids* **2004**, 9, 2005.
